# Supplementary material for: How Much is 131 Million Dollars? Putting Numbers in Perspective with Compositional Descriptions
Source: arXiv:1609.00070 source file (2016-09-01)
Supplement: Supplementary file 1 [file appendix.tex]

\section{Knowledge base}
\label{sec:kb}

\input tupledb.table
